# Supplementary material for: BO-Muse: A human expert and AI teaming framework for accelerated experimental design
Source: arXiv:2303.01684 source file (2023-03-30)
Supplement: Supplementary file 1 [file Supplementary_Arun.tex]

%In addition to the experimental results mentioned in the main paper,
%we provide the optimisation performance of our proposed BO-Muse framework
%on Rastrigin-5D function. The details of Rastrigin-5D synthetic function is mentioned in Table \ref{tab:syn_details_sup}.
%
%We maintain the same experimental settings mentioned in the main paper
%for the additional experiment conducted. For a given $d$ dimensional problem, we use $d+1$ initial observations and optimise for $10\times d$ iterations i.e., the budget allocated for our synthetic experiments is set to $10\times d$ function evaluations. The simple regret plot
%obtained for Rastrigin-5D function after 10 runs with random initialisations are shown in Figure \ref{fig:rastrigin5d}. 
%
%\begin{table}[h]
%\centering{}{\footnotesize{}}%
%\begin{tabular}{ccc}
%\toprule 
%Functions & $f^{\star}(\mathbf{x})$ & High Level Features\tabularnewline
%\midrule
%\multirow{2}{*}{Rastrigin-5D} & \multirow{2}{*}{$10d+\sum_{i}^{d}[{x}_{i}^{2}-10\cos(2\pi{x}_{i})]$ 
%$\forall i\in\mathbb{N}_{5}$} & ${x}'_{i}={x}_{i}^{2}$ $\forall i\in\mathbb{N}_{5}$\tabularnewline
% &  & ${x}'_{j+5}=\cos{x}_{j}$ $\forall j\in\mathbb{N}_{5}$\tabularnewline
%\bottomrule
%\end{tabular}\caption{Synthetic optimisation benchmark functions. Analytical forms are provided
%in the second column and the last column depicts the features used
%by a simulated human expert.}
%\label{tab:syn_details_sup}
%\end{table}
%
%\begin{figure}
%\begin{centering}
%\par\end{centering}
%\begin{centering}
%\includegraphics[width=0.44\columnwidth]{Images/Regret_Rastrigin}
%\caption{Simple regret vs iterations for Rastrigin-5D synthetic function. We plot the mean regret along with its standard error after 10 runs with random initialisations.\label{fig:rastrigin5d}}
%\par\end{centering}
%\end{figure}
